# Supplementary material for: Honeypot Implementation in a Cloud Environment
Source: arXiv:2301.00710 source file (2024-07-17)
Supplement: Supplementary file 1 [file appendix.tex]

%\chapter*{SSH Honeypot}
%\lstset{basicstyle=\ttfamily, style=thesis}

%\lstinputlisting[language=c, title={auth-passwd.c}, label={lst:auth-passwd}]{listings/auth-passwd.c}

%\lstinputlisting[language=c, title={auth.c}, label={lst:auth}]{listings/auth.c}

%\lstinputlisting[language=c, title={channels.c}, label={lst:channels}]{listings/channels.c}

%\lstinputlisting[language=c, title={misc.h}, label={lst:misc}]{listings/misc.h}

%\lstinputlisting[language=c, title={serverloop.c}, label={lst:serverloop}]{listings/serverloop.c}

%\lstinputlisting[language=c, title={sshd.c}, label={lst:sshd}]{listings/sshd.c}
